# Supplementary material for: Revisiting Initialization of Neural Networks
Source: arXiv:2004.09506 source file (2020-06-04)
Supplement: Supplementary file 1 [file appendix.tex]

\section*{APPENDIX}

\subsection{Proof of Hessian Chain Rule}
Our goal is to compute the Hessian with respect to the parameters in the layer $k$. %We first obtain formulas with respect to the output $z^{(k+1)}$. 
By the chain rule
\begin{align}
   D_{w^{(k)}}L = D_{ z^{(n)}} L \bullet D_{w^{(k)}} z^{(n)} 
\end{align}
Note that the second tensor is of shape $[d_n,d_{k+1},d_k]$ (rank 3!), the contraction is over the dimension of $z^{(n)}$. Again by the chain and product rules
\begin{align}\label{eq:hessian_1}
  D^2_{w^{(k)} } L = \underbrace{ D^2_{ z^{(n)}} L \bullet D_{w^{(k')}} z^{(n)}  \bullet D_{w^{(k)}} z^{(n)} }_{H_1} + \underbrace{D_{ z^{(n)}} L \bullet D^2_{w^{(k)}} z^{(n)} }_{H_2}
\end{align}
In the component $H_1$ the dot-products contract indices $z^{(n)}$ (note that $D^2$ is symmetric and the terms $D$ are same, hence the order of pairing dimensions of $w^{(k)}$ does not matter). As for the second component $H_2$, it is a product of tensors of rank $1$ and $5$. In order to further simplify, we are going to show that $H_2$ negligible compared to $H_1$. the intuition is as follows:
in $H_1$ the contribution comes from gradients $D_{w^{(k)}}$ while in $H_2$ from second-order derivatives $D^2_{w^{(k)}}$; we consider activations such that $f(u) = au+O(u^3)$ and therefore for small $u$ second-derivatives are near zero but first derivatives are not, and their contributions dominate.

In the analysis below we assume that weights are sufficiently small, and biasses are zero (or of much smaller variance compared to weights). 
Let $u^{(k)} = w^{(k)}\cdot z^{(k)} + b^{(k)}$ be the output before activation at the $k$-th layer.

Due to \Cref{eq:hessian_1}, our goal is to evaluate first and second derivatives of $z^{(n)}$ with respect to weights $w^{(k)}$, under the assumption that inputs $z^{(i)}$ are sufficiently small. Consider how $z^{(k+1)}$ depends on $w^{(k)}$.
By the chain rules
\begin{align}\label{eq:expansion1}
D_{w^{(k)}} z^{(k+1)} & = D_{u^{(k)}} f(u^{(k)})\bullet D_{w^{(k)}} u^{(k)} \\
D^2_{w^{(k)}} z^{(k+1)} & = D^2_{u^{(k)}} f(u^{(k)})\bullet D_{w^{(k)}} u^{(k)} \bullet D_{w^{(k)}} u^{(k)} 
\end{align}
Note that $D_{u^{(k)}} f(u^{(k)})$ and $D^2_{u^{(k)}} f(u^{(k)})$ are diagonal tensors because $f$ is applied element-wise.
More precisely
\begin{align}\label{eq:expansion2}
\left[D^2_{u^{(k)}} f(u^{(k)})\right]_{i,j,j'}= \delta_{i,j}\delta_{i,j'}\cdot f''(u^{(k)}_i) 
\end{align}
where $\delta_{\cdot,\cdot}$ is the Kronecker delta which is one where indices match and zero otherwise. 
Moreover,
\begin{align}\label{eq:expansion3}
\left[D_{w^{(k)}} u^{(k)}\right]_{j,p,q} = \frac{\partial}{\partial w^{(k)}_{p,q}} (w^{(k)}\cdot z^{(k)}+b^{(k)})_j = \delta_{j,p}\cdot z^{(k)}_{q}
\end{align}
Thus
\begin{align}
\left[D^2_{w^{(k)}} z^{(k+1)}\right]_{i,p,q,p',q'} =  \delta_{i,p}\delta_{i,p'} \cdot f''(u^{(k)}_{i}) \cdot z^{(k)}_{q}\cdot z^{(k)}_{q'}
\end{align}
When this tensor acts, as a bi-linear form, on a tensor $g = g_{p,q}$ we therefore obtain
\begin{align}
\left[D^2_{w^{(k)}} z^{(k+1)}\bullet g \bullet g\right]_i &=   f''(u^{(k)}_i) \sum_{q,q'} z^{(k)}_{q} z^{(k)}_{q'} g_{i,q} g_{i,q'} \\
& = f''(u^{(k)}_i)\left(\sum_{q} z^{(k)}_q g_{i,q}\right)^2
\end{align}
Since our assumption on activations implies $f''(u) = O(f'''\cdot u)$ for real $u$, we see this is of order $O(f'''\|u^{(k)}\|\|z^{(k)}\|^2)\cdot\|g\|^2$.
\begin{claim}[Magnitude of second derivative of weights]
\begin{align}
D^2_{w^{(k)}} z^{(k+1)}\bullet g \bullet g =   O(f'''\|u^{(k)}\|\|z^{(k)}\|^2)\cdot\|g\|^2.
\end{align}
which is of order $O(f'''\cdot c^3)$ where $c$ is the constant from our 'relatively small inputs' assumption.
\end{claim}
Next, observe that the roles of $z^{(k)}$ and $w^{(k)}$ in $u^{(k)}$ are symmetric. Thus we have a similar result with respect to $z^{(k)}$.
\begin{claim}[Magnitude of second derivative of inputs]
\begin{align}
D^2_{z^{(k)}} z^{(k+1)}\bullet g \bullet g =   O(f'''\|u^{(k)}\|\|w^{(k)}\|^2)\cdot\|g\|^2
\end{align}
which is of order $O(f'''\cdot c)$ where $c$ is the constant from our 'relatively small inputs' assumption.
\end{claim}

We need to prove that this propagates to higher-level outputs $z^{i}$, where $i>k$. This is intuitive, 
considering now that $z^{(i)}$ is a function of $z^{(k+1)}$ with no dependencies on $w^{(k)}$. To prove it formally look at the second-order chain rule
\begin{align}
D^{2}_{w^{(k)}} z^{(i)} = D^2_{z^{(k+1)}}{z^{(i)}}\bullet D_{w^{(k)}} z^{(k+1)} \bullet D_{w^{(k)}} z^{(k+1)} + D_{z^{(k+1)}} z^{(i)}\bullet D^{2}_{w^{(k)}}z^{(k+1)}
\end{align}
Now the second term is clearly $O(f'''c^3)$ by the first claim. As for the first term, the first tensor is of order $O(f'''c)$ while 
the two others are $O(f'c)$. The dot-product gives the bound $O(f'''c^3)$.
\begin{claim}
For every $i>k$ it holds $D^{2}_{w^{(k)}} z^{(i)} = O(f''c^3)$.
\end{claim}

Summing up, we can ignore second-derivatives with respect to weights, and this is accurate except third-order terms in the magnitude of $z^{(i)}$. In particular, we can ignore the effect of $H_2$.

\subsection{Factorizing the Hessian Quadratic Form}
Consider any potential update vector $g$ for weights $w^{(k)}$, it has to be of same shape as $D_{w^{(k)}}L$ or quivalently $w^{(k)}$, that is $[d_{k+1},d_{k}]$. Our goal is to evaluate the hessian quadratic form on $g$. Ignoring the smaller part $H_2$ we are left with $H_1$ which gives 
\begin{align}\label{eq:hessian_3}
   D^2_{w^{(k)}}L\bullet g \bullet g = D^2_{ z^{(n)}} L \bullet D_{w^{(k)}} z^{(n)} \bullet D_{w^{(k)}} z^{(n)} \bullet g \bullet g
\end{align}
where $g$ is contracted on all indices together with $w^{(k)}$.
To emphasize this we can regroup, obtaining
\begin{claim}[Hessian quadratic form]
The hessian quadratic form for an update $g$ equals
\begin{align}\label{eq:hessian_4}
D^2_{w^{(k)}}L\bullet g \bullet g = D^2_{ z^{(n)}} L \bullet \left( D_{w^{(k)}} z^{(n)} \bullet g\right) \bullet \left( D_{w^{(k)}} z^{(n)} \bullet g\right)
\end{align}
\end{claim}
We work further to simplify rank-3 tensors. By the chain rule
\begin{align}\label{eq:action_gradient}
D_{w^{(k)}} z^{(n)}\bullet g = D_{z^{(k+1)}} z^{(n)}\bullet D_{w^{(k)}} z^{(k+1)} \bullet g
\end{align}
Let $u^{(k)} = w^{(k)}\cdot z^{(k)} + b^{(k)}$ be the output before activation. By the chain rule
\begin{align}\label{eq:action_gradient_2}
D_{w^{(k)}} z^{(k+1)}  = D_{u^{(k)}} {z^{(k+1)}}\bullet D_{w^{(k)}} u^{(k)}  
\end{align}
Note that $D_{w^{(k)}} u^{(k)} $ is a third-order tensor of shape $[d_{k+1},d_{k+1},d_{k}]$. Denote its elements by $M_{i',i,j}$. We have
\begin{align}
\left[D_{w^{(k)}} u^{(k)}\right]_{i',i,j} = [i'=i]\cdot z^{(k)}_{j}
\end{align}
and we compute the dot product
\begin{align}
\left[D_{w^{(k)}} u^{(k)} \bullet g \right]_{i'} = \sum_{i,j} \left[D_{w^{(k)}} u^{(k)}\right]_{i',i,j}g_{i,j} =  \sum_j z^{(k)}_{j} g_{i',j} 
\end{align}
which can be expressed compactly in terms of matrix multiplication as
\begin{align}\label{eq:action_gradient_3}
D_{w^{(k)}} u^{(k)} \bullet g = g\cdot z^{(k)}
\end{align}
which is a vector of shape $[d_{k+1}]$. 
%We can estimate its spectral norm as 
%\begin{align}\label{eq:action_gradient_norm_1}
%\left\|D_{w^{(k)}} u^{(k)} \bullet g\right\| = \| g\cdot z^{(k)}\| \leqslant \|g\| \cdot \|z^{(k)}\|
%\end{align}
Using this in \Cref{eq:action_gradient_2} we obtain, in terms of matrix products
\begin{align}
D_{w^{(k)}} z^{(k+1)}  \bullet g = D_{u^{(k)}} {z^{(k+1)}} \cdot  \left( D_{w^{(k)}} z^{(k+1)}  \bullet g\right) = D_{u^{(k)}} {z^{(k+1)}}\cdot g\cdot z^{(k)}
\end{align}
%Since the norm is sub-multiplicative by \Cref{eq:action_gradient_norm_1} we have
%\begin{align}\label{eq:action_gradient_norm_2}
%\|D_{w^{(k)}} z^{(k+1)}  \bullet g\| \leqslant \| D_{u^{(k)}} {z^{(k+1)}} \| \cdot \| g\|\cdot \|z^{(k)}\| 
%\end{align}
Now, in terms of matrix products, \Cref{eq:action_gradient} becomes
\begin{align}
D_{w^{(k)}} z^{(n)}\bullet g =  D_{z^{(k+1)}} z^{(n)}\cdot D_{w^{(k)}} z^{(k+1)}  \cdot g \cdot z^{(k)}
\end{align}
which is a vector of shape $[d_n]$. Finally note that $H\bullet v \bullet v =v^T\cdot  H\cdot v$ where $H$ is a symmetric matrix and $v$ is vector.  This proves
\begin{claim}[Approximated hessian form]
For sufficiently small inputs, the hessian quadratic form can be approximated as
\begin{align}
\mathbf{H}_{w^{(k)}}[g,g] \approx v^T\cdot \mathbf{H}_z \cdot  v
\end{align}
where 
\begin{align}
v=D_{z^{(k+1)}} z^{(n)}\cdot D_{w^{(k)}} z^{(k+1)}  \cdot g \cdot z^{(k)}.
\end{align}
\end{claim}
This claim implies the first part of \Cref{thm:hessian_chainrule}. The error estimate follows by follows by the discussion in the previous subsection.

\subsection{Further Factorization}

We have seen that the quadratic effects of $w^{(k)}$ can be ignored, thus it is enough to consider the simplified recursion
\begin{align}
z^{(k+1)} \approx a \cdot \left(w^{(k)}\cdot z^{(k)} + b^{(k)}\right) 
\end{align}
for a diagonal matrix $a$ (which captures first-derivatives of activations), or equivalently:
\begin{claim}[Second-order recursion for small inputs]
For relatively small inputs the hessian can be computed under the simplified recursion
\begin{align}
z^{(k+1)} \approx \mathbf{J}^{(k)}\cdot  z^{(k)}
\end{align}
where $\mathbf{J}^{k} = D_{z^{(k)}}z^{(k+1)}$. In particular the term $H_2$ can be ignored.
\end{claim}

We now proceed to further factorize $v$. 
By linearization we obtain
\begin{align}
z^{(k)} \approx  D_{z^{(k-1)}}  z^{(k)} \cdot z^{(k-1)} = \ldots = D_{z^{(k-1)}}  z^{(k)} 
\end{align}
Moreover, by the chain rule, output gradient facatorizes as 
\begin{align}
 D_{z^{(k+1)}}z^{(n)} =  D_{z^{(n-1)}}z^{(n)}\cdot z^{(k-1)} \cdot D_{z^{(n-2)}}z^{(n-1)}\cdot \ldots \cdot  D_{z^{(k+1)}}z^{(k+2)}
\end{align}
regardless of linearizing assumptions. Combining these two observations gives
\begin{claim}[Factorizing under linearization]
Up to terms linear in $z^{(i)}$ for $i=k-1,\ldots,1$ we have
\begin{multline}
v \approx D_{z^{(n-1)}}z^{(n)}\cdot  D_{z^{(n-2)}}z^{(n-1)}\cdot \ldots \cdot  D_{z^{(k+1)}}z^{(k+2)} \cdot A \cdot g \\
 \cdot D_{z_{(k-1)}}z^{(k)}\cdot \ldots D_{z^{(0)}}z^{(1)}\cdot z^{(0)}
\end{multline}
\end{claim}
This proves \Cref{eq:full_factorization}.

%The spectral norm is sub-multiplicative, which means that the norm of a matrix product is at most the product of norms. This implies the first part of \Cref{thm:hessian_bound}. 
%so that, with $v$ as in \Cref{thm:hessian_chainrule} we have approximately
%which proves the second part.

%\begin{align}
 %   \frac{\partial^2 L}{\partial x\partial x'} = \frac{\partial^2 L}{\partial z^n \partial {z^n}^{'}}\prod \frac{\partial z^j}{\partial z^{j-1}}\frac{\partial {z'}^j}{\partial {z'}^{j-1}}
%\end{align}
%Using the spectral norm we can estimate
%\begin{align}
%\left\|    \frac{\partial^2 L}{\partial x\partial x'}  \right\| \leqslant \left\| \frac{\partial^2 L}{\partial z^n \partial {z^n}^{'}}\right\|\cdot \prod_i \|w^i\|^2
%\end{align}
